# Supplementary material for: 3d $\mathcal{N}=4$ mirror symmetry with 1-form symmetry
Source: arXiv:2301.02409 source file (2023-04-13)

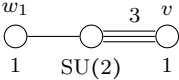

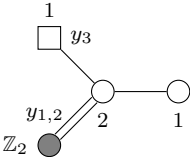

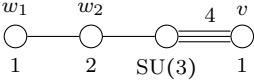

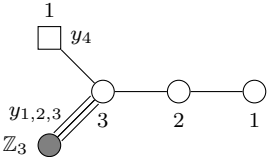

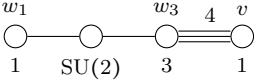

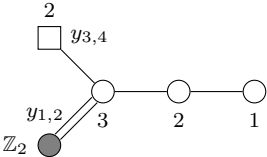

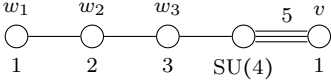

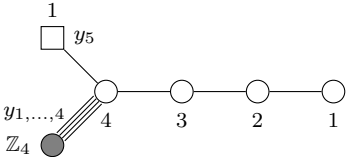



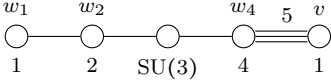

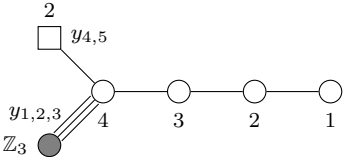

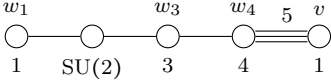

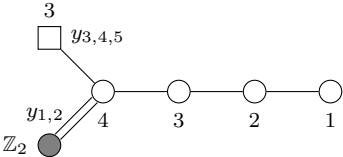

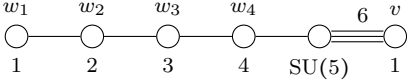

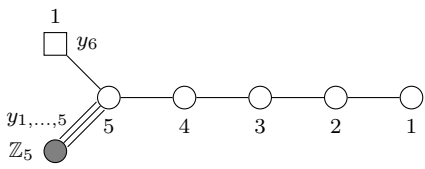

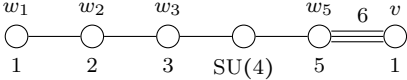

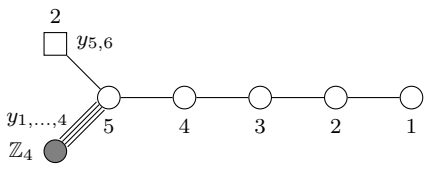



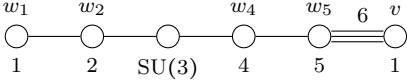

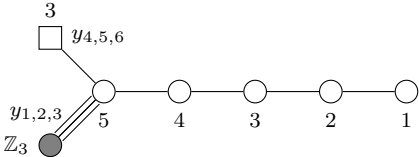

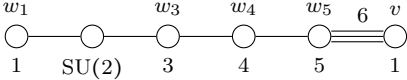

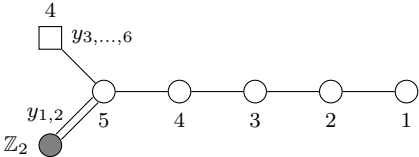

Supplement: Supplementary file 1 [file figures_1-form_appendix.pdf]
